# Supplementary material for: Dynamical structure factors and excitation modes of the bilayer Heisenberg model
Source: arXiv:1508.07816 ancillary file (2015-08-31)
Supplement: Supplementary file 1 [file SM.pdf]

# Dynamical structure factors and excitation modes of the bilayer Heisenberg model
# Supplemental Material

M. Lohöfer,[1] T. Coletta,[2] D. G. Joshi,[3] F. F. Assaad,[4] M. Vojta,[3] S. Wessel,[1] and F. Mila[5]

[1] *Institut für Theoretische Festkörperphysik, JARA-FIT and JARA-HPC, RWTH Aachen University, 52056 Aachen, Germany*
[2] *School of Engineering, University of Applied Sciences of Western Switzerland, 1951 Sion, Switzerland*
[3] *Institut für Theoretische Physik, Technische Universität Dresden, 01062 Dresden, Germany*
[4] *Institut für Theoretische Physik und Astrophysik, Universität Wüzburg, Am Hubland, 97074 Würzburg, Germany*
[5] *Institute of Theoretical Physics, Ecole Polytechnique Fédérale de Lausanne (EPFL), 1015 Lausanne, Switzerland*

(Dated: August 4, 2015)

The bilayer Heisenberg model is an effective low energy model describing the spin dynamics of Mott insulators. In this supplemental material, we show that the spin dynamics obtained from simulations of the Heisenberg model can be obtained by starting from the Hubbard model on the bilayer square lattice. At intermediate couplings, this is by no means trivial since charge fluctuations allow for higher order spin exchange processes. Our starting point reads:

$$H = -\sum_{\boldsymbol{i},\boldsymbol{j},\sigma} c^{\dagger}_{\boldsymbol{i},\sigma} T_{\boldsymbol{i},\boldsymbol{j}} c_{\boldsymbol{j},\sigma} + \frac{U}{2}\sum_{\boldsymbol{i}} \left(n_{\boldsymbol{i}} - 1\right)^2 . \tag{1}$$

Here, $c^{\dagger}_{\boldsymbol{i},\sigma}$ creates an electron in Wannier state centered around lattice site $\boldsymbol{i}$ and with $z$-component of spin $\sigma$, $T_{\boldsymbol{i},\boldsymbol{j}}$ accounts for in-plane hopping of magnitude $t$ between nearest neighbors as well as an interlayer hoping set by $t'$. Finally, double occupancy of Wannier states is prohibited by the Hubbad term, with $n_{\boldsymbol{i}} = \sum_{\sigma} c^{\dagger}_{\boldsymbol{i},\sigma} c_{\boldsymbol{i},\sigma}$

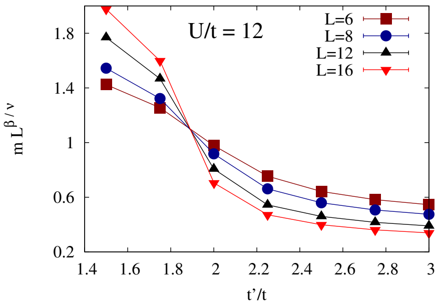


FIG. 1. Finite size scaling assuming 3D $O(3)$ critical exponents [1], $\nu = 0.7048(30)$ and $\beta = 0.3616(31)$

At the particle-hole symmetric point, one can carry out sign free quantum Monte Carlo simulations of the model. Here, we have used the projective zero temperature approach based on the equation,

$$\frac{\langle \Psi_0 | O | \Psi_0 \rangle}{\langle \Psi_0 | \Psi_0 \rangle} = \lim_{\Theta \to \infty} \frac{\langle \Psi_T | e^{-\Theta H} O e^{-\Theta H} | \Psi_T \rangle}{\langle \Psi_T | e^{-2\Theta H} | \Psi_T \rangle}, \tag{2}$$

in which the ground state is filtered out of a single slater determinant by propagating along the imaginary time axis. It is beyond the scope of this supplemental material to go into the details of the implementation and the reader is referred to Ref. [2] for an overview of the algorithm. Let us however comment on some aspects of our implementation. We have used an $SU(2)$-spin symmetric discrete Hubbard-Stratonovitch transformation coupling to the charge:

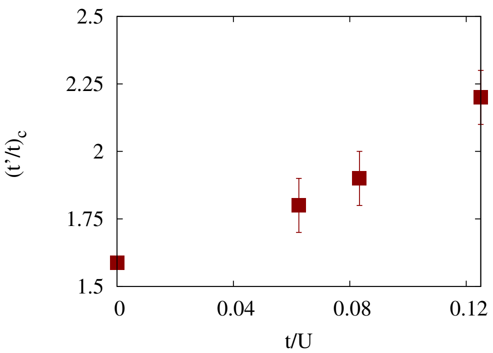


FIG. 2. Critical value of $t'$ as a function of the Hubbard interaction. The data point at $U/t \to \infty$ corresponds to the Heisenberg result

$$e^{-\Delta\tau U (n_i - 1)^2/2} = \frac{1}{2}\sum_{s=\pm 1} e^{i\alpha s (n_i - 1)}, \tag{3}$$

with $\cos(\alpha) = e^{-\Delta\tau U/2}$. We have furthermore used a symmetric Trotter decomposition with $\Delta\tau U = 0.8$ and the trial wave function corresponds to the ground state of the non-interacting Hamiltonian. Here, parameters were chosen so as to avoid a degenerate ground state for the non-interacting system. Thereby, the trial wave function is a spin-singlet, and due to Liebs theorem [3] in the correct symmetry sector of the ground state of the bilayer Hubbard model. For this spin singlet trial wave function projection parameters $\Theta t = 40$ suffice to guarantee convergence to the ground state within the quoted accuracy.

In the strong coupling limit, second order perturbation in $t/U$ yields $J = 4t^2/U$ and $J' = 4t'^2/U$ such that the Heisenberg result $g_c \equiv (J'/J)_c = 2.5220(1)$ translates to $(t'/t)_c = 1.59$ as $U/t \to \infty$. To determine the critical

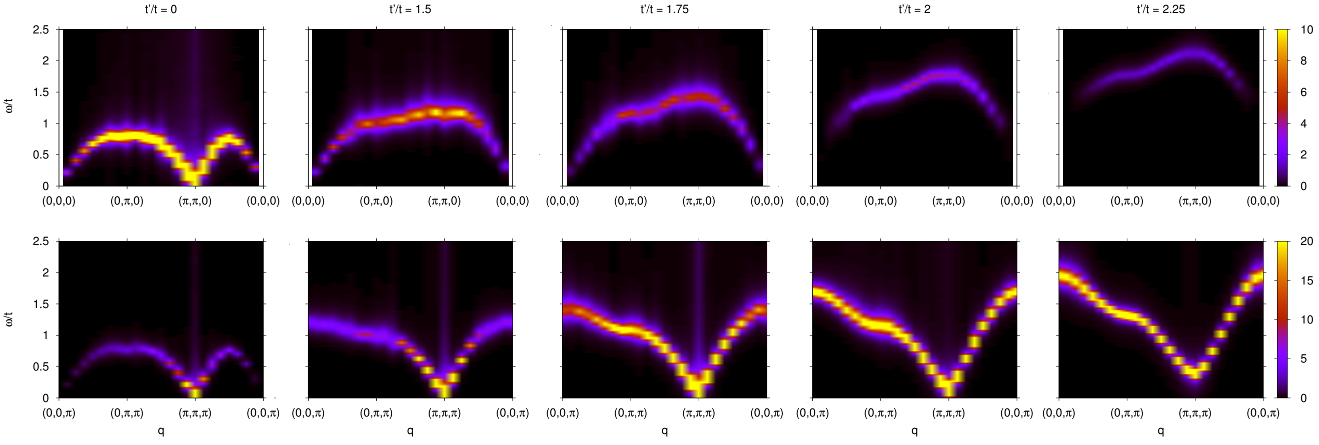


FIG. 3. Dynamical spin structure factor at $U/t = 12$ across the quantum phase transition. For this value of the Hubbard interaction $(t'/t)_c = 1.9 \pm 0.1$. The numerical simulations were carried out with a spin singlet trial wave function.

value of of $t'$ we have used the finite size scaling Ansatz:

$$m = L^{-\beta/\nu} F(|t'_c - t'|L^{1/\nu}) \tag{4}$$

with magnetization

$$m = \sqrt{\langle \boldsymbol{S_Q S_{-Q}} \rangle}. \tag{5}$$

Here $\boldsymbol{S_q} = \sqrt{\frac{1}{2L^2}} \sum_{\boldsymbol{i}} e^{i\boldsymbol{q}\cdot\boldsymbol{i}} \boldsymbol{S_i}$, with $\boldsymbol{S_i} = \frac{1}{2}\sum_{s,s'} c^{\dagger}_{\boldsymbol{i},s} \boldsymbol{\sigma}_{s,s'} c_{\boldsymbol{i},s'}$ the spin-1/2 operator, $L$, the linear size of the lattice and $\boldsymbol{Q} = (\pi,\pi,\pi)$, the antiferromagnetic wave vector. Fig. 1 shows the finite size scaling of the magnetization using the three dimensional $O(3)$ critical exponents [1]. As apparent, $(t'/t)_c = 1.9 \pm 0.1$ at $U/t = 12$. Similar results allow us to pin down the value of $(t'/t)_c$ as a function function of $U/t$. The data, see Fig. 2, is consistent, as expected, with $t'_c$ extrapolating to the Heisenberg value as $U/t \to \infty$. A similar analysis was carried out in Ref. [4].

To compare with the Heisenberg results, we have computed the dynamical spin structure factor which in the Lehmann representation reads:

$$S(\boldsymbol{q},\omega) = 2\pi \sum_n |\langle n|\boldsymbol{S_q}|0\rangle|^2 \delta(\omega - E_n - E_0). \tag{6}$$

The sum

$$\int d\omega S(\boldsymbol{q},\omega) = 2\pi \langle \boldsymbol{S_q} \cdot \boldsymbol{S_{-q}} \rangle \tag{7}$$

relates the static and dynamical spin structure factors. In analogy to the results produced for the Heisenberg model, we have used the stochastic analytical continuation described in Ref. [5] to carry out the Wick rotation.

Fig. 3 shows the dynamical spin structure factor across the quantum phase transition at $U/t = 12$ on an $L = 16$ lattice. For this value of the $U/t$ the single particle gap is of the order of $\Delta_s \simeq 4t$ such that the particle-hole continuum should become apparent as of $2\Delta_s \simeq 8t$. From the sum-rule it becomes apparent that the great majority of the spectral weight lies in magnon excitations. Comparison with Sec. III A of the article shows that the overall evolution of dynamical spin structure factor is very similar, if not identical, to the QMC results for the Heisenberg bilayer.

[1] K. Chen, A. M. Ferrenberg, and D. P. Landau, Phys. Rev. B **48**, 3249 (1993).

[2] F. Assaad and H. Evertz, in *Computational Many-Particle Physics*, Vol. 739 of *Lecture Notes in Physics*, edited by H. Fehske, R. Schneider, and A. Weiße (Springer, Berlin Heidelberg, 2008), pp. 277–356.

[3] E. H. Lieb, Phys. Rev. Lett. **62**, 1201 (1989).

[4] M. Golor, T. Reckling, L. Classen, M. M. Scherer, and S. Wessel, Phys. Rev. B **90**, 195131 (2014).

[5] K. S. D. Beach, arXiv:0403055 (2004).
